# Supplementary material for: Enhanced Kalman with Adaptive Appearance Motion SORT for Grounded Generic Multiple Object Tracking
Source: arXiv:2410.09243 source file (2024-10-11)
Supplement: Supplementary file 1 [file X_suppl.tex]

\textcolor{red}{DO NOT INCLUDE MUCH TEXT. THIS IS NOT ANOTHER SUBMISSION - Shrinking the text (Duy)}

In this supplementary section, we will explore several key aspects in detail. To begin with, we will provide details on G$^2$MOT dataset with an overall of G$^2$MOT in Section \ref{sec:overall}, an in-depth explanation of the data annotation procedure in Section \ref{sec:anno_proc}, data structure in Section \ref{sec:data_structure} and statistical insights of G$^2$MOT in Section \ref{sec:statis}. Then, we will present intuitions of the proposed Kalman++ together ablation study on Kalman++ in Section \ref{sec:kalman}. Additionally, we will showcase additional qualitative results in Section \ref{sec:quali}. Finally, we will include some discussion on Grounded GMOT.

\section{G$^2$MOT Dataset}
\label{sec:data}
\subsection{Overall}
\label{sec:overall}
Unlike conventional GMOT datasets, the G$^2$MOT evaluation protocol is clearer and free of ambiguity when compared with previous datasets relying on the one-shot protocol. To achieve this goal, we introduce a textual description during the annotation process and use it to clarify the exact characteristics of the set of objects we want to track.  \textcolor{red}{this was in the main paper already}
%, as demonstrated in Figure \ref{fig:fig_supp_w_anno1} and Figure \ref{fig:fig_supp_w_anno2}.

In terms of dataset challenges, we have found that most of the current datasets already provide a wide range of challenging tasks for object tracking. Hence, instead of collecting new videos, we are using the existing tracking ground truth and annotating it to match our problem setup. As a result, our dataset not only covers a wide range of challenging videos but also increases the difficulty level by requiring solutions to understand the fine-grained characteristics of objects instead of just their category.

\subsection{Data Annotation Procedure}
\label{sec:anno_proc}

Our approach does not gather new videos but instead enriches existing datasets like GMOT-40 \cite{bai2021gmot}, AnimalTrack \cite{zhang2022animaltrack}, DanceTrack \cite{sun2022dancetrack}, and SportMOT \cite{cui2023sportsmot} with textual descriptions, diversifying the scope of generic multiple object tracking (MOT). While GMOT-40 and AnimalTrack focus on various object categories, DanceTrack and SportMOT pivot to human-centric themes, such as team dances and sports competitions, where distinguishing individuals in similar attire poses a significant challenge. This blend, including human activities, different animal species, and scenarios with rapid movements, enriches our G$^2$MOT dataset. It introduces complexities like camera dynamics, size variability, occlusions, scale changes, and motion blur, making it robust for tracking studies. The dataset's integrity is upheld by extensive manual annotations from a team of four professionals and a thorough double-checking procedure to guarantee annotation accuracy and consistency \cite{bai2021gmot, zhang2022animaltrack, sun2022dancetrack, cui2023sportsmot}.

\subsection{Data Structure}
\label{sec:data_structure}
Our annotation consists of two parts corresponding to textual description annotation and tracking annotation as introduced in Section 3.2 (main paper). In particular, the annotation format of JSON files is as follows:

\begin{lstlisting}[language=json, caption={Annotation format of G$^2$MOT dataset.}, label={lst:anno_fmt}]
{
  "videos": [video],
  "tracking_queries": [tracking_query]
}
video{
    "id": int,
    "video_path": str
}
tracking_query{
    "id": int,
    "video_id"; int,
    "class_name": str,
    "type": str, #"superset" or "subset"
    "synonyms": [str],
    "definition": str,
    "attributes": [str],
    "track_path": str,
    "caption": str,
}
\end{lstlisting}

A full annotation is shown in Figure \ref{fig:data_annotation} whereas the textual description is further illustrated in Figure \ref{fig:fig_supp_w_anno}.

\begin{figure*}
    \centering
    \includegraphics[width=\textwidth]{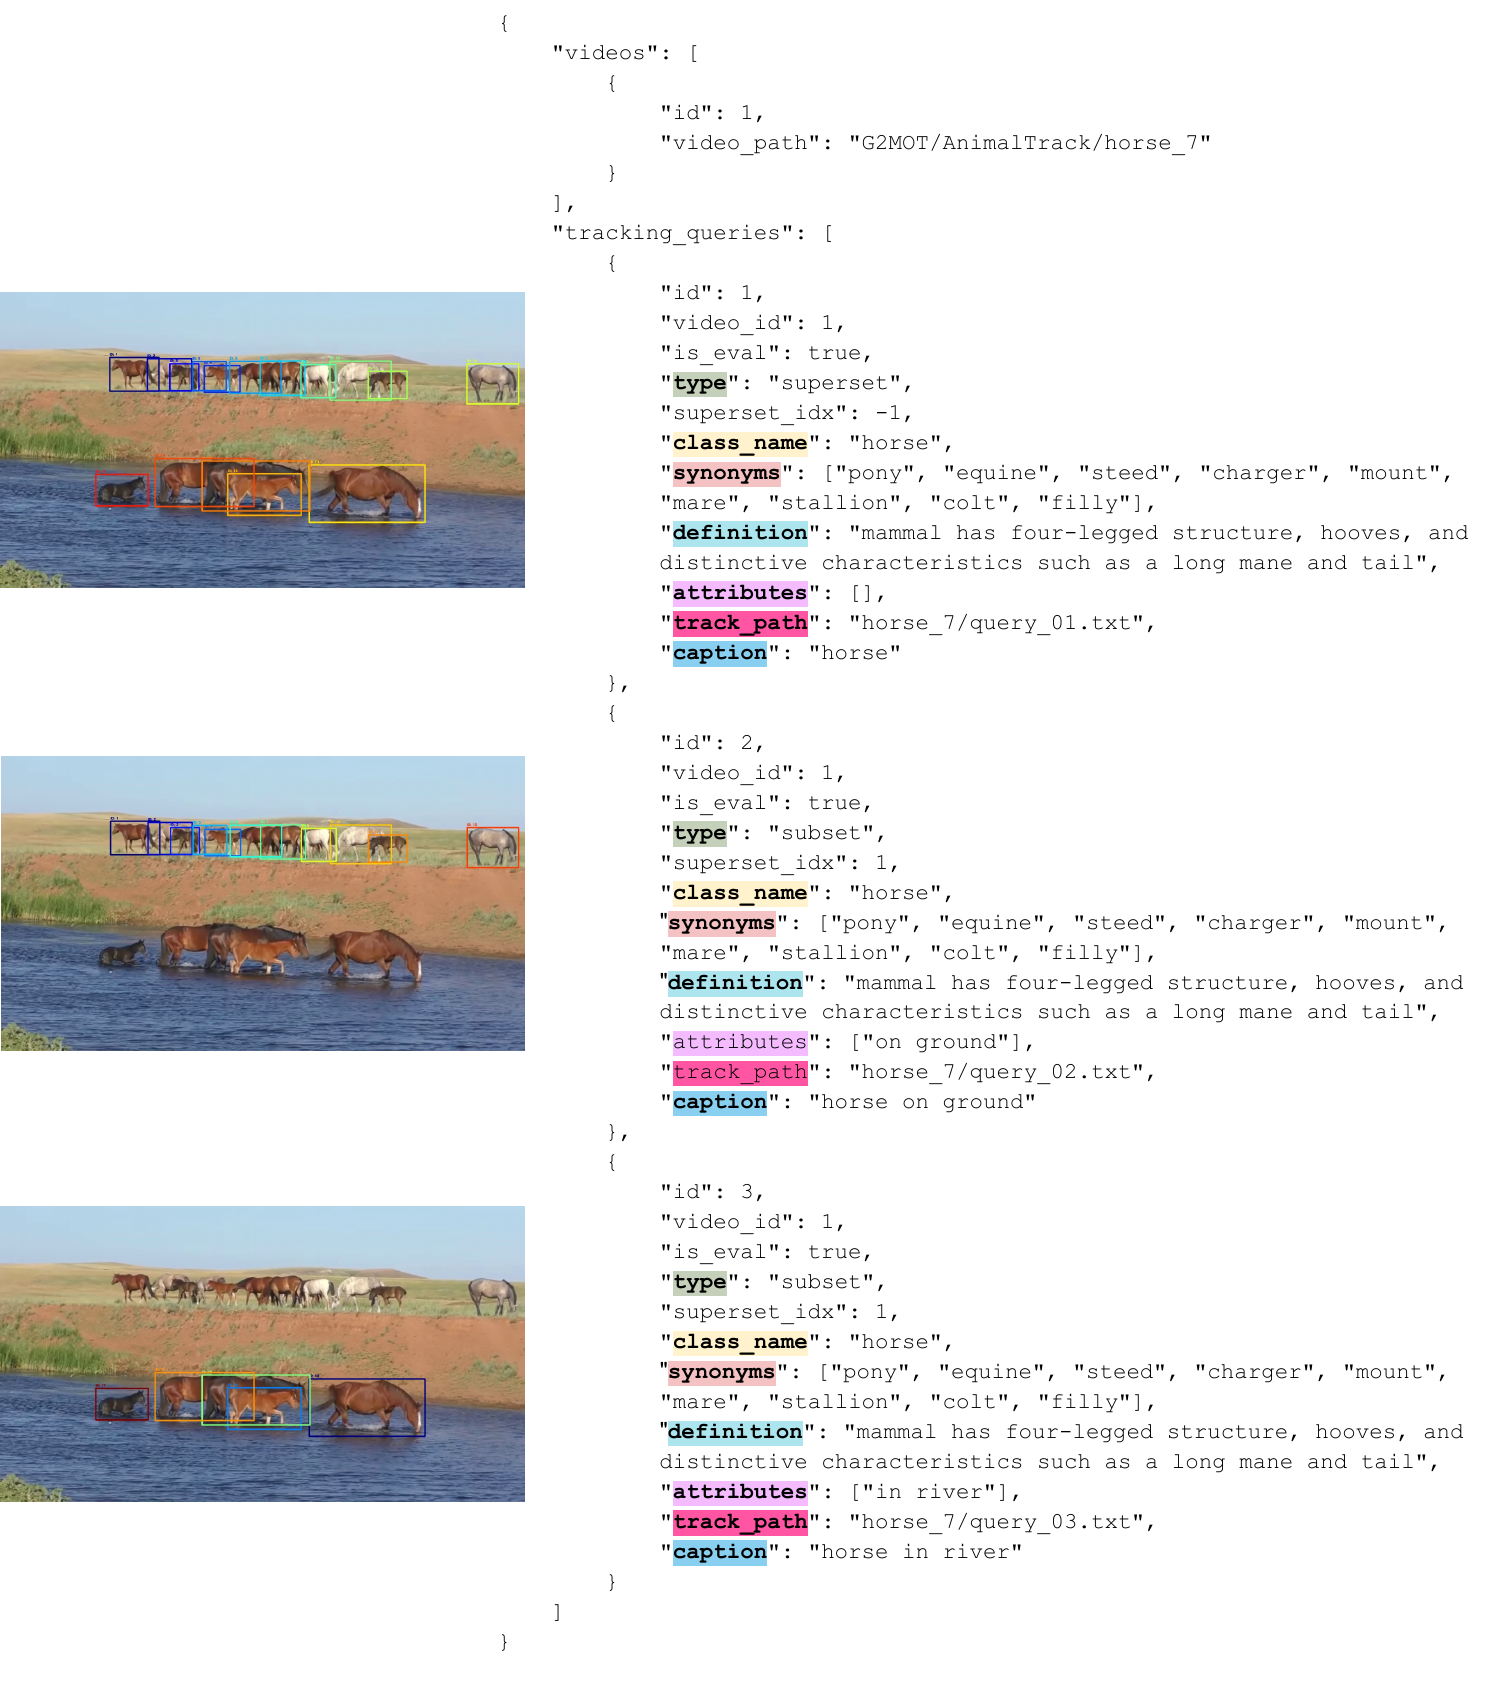}
    \caption{As an illustration of our annotation, consider the video "horse\_7." It includes one superset representing all horses within the scene and two subsets that specifically identify horses on the ground and horses in the river.}
    \label{fig:data_annotation}
\end{figure*}

\begin{figure*}
    \centering
    \includegraphics[width=\linewidth]{figures/supp/[sup]dataset_sample_with_annotate.pdf}
    \caption{Demonstration of textual description within the same video.}
    \label{fig:fig_supp_w_anno}
\end{figure*}

% \begin{figure*}
%     \centering
%     \includegraphics[width=\linewidth]{figures/supp/[sup]dataset_sample_with_annotate_2.pdf}
%     \caption{Additional demonstration of textual description in Section \ref{sec:anno}.}
%     \label{fig:fig_supp_w_anno2}
% \end{figure*}

\subsection{Statistical Insights of G$^2$MOT}
\label{sec:statis}

\begin{wraptable}{r}{0.4\linewidth}
\vspace{-100}
\centering
\setlength{\tabcolsep}{2pt}

    \centering
    \caption{Statistics insights of G$2$MOT. \# denotes the quantity of the respective items.}
    \resizebox{\linewidth}{!}{\begin{tabular}{lrrr}
        \toprule
        \textbf{Class Name} & \# \textbf{Frames} & \# \textbf{Objects} & \# \textbf{Boxes} \\
        \midrule
        ant & 302 & 72 & 4668 \\
        airplane & 1181 & 81 & 23307 \\
        athlete & 90642 & 1282 & 591146 \\
        balloon & 3218 & 557 & 83430 \\
        ball & 729 & 181 & 20399 \\
        bee & 357 & 225 & 9439 \\
        bird & 3462 & 307 & 70972 \\
        boat & 1472 & 143 & 29491 \\
        car & 2023 & 221 & 33893 \\
        chicken & 7615 & 226 & 54710 \\
        deer & 2762 & 222 & 53339 \\
        dolphin & 1718 & 167 & 31112 \\
        duck & 4851 & 277 & 79416 \\
        fish & 569 & 291 & 21922 \\
        goose & 1773 & 195 & 33120 \\
        horse & 6556 & 281 & 69524 \\
        penguin & 1844 & 137 & 30312 \\
        person & 83623 & 939 & 688535 \\
        pig & 1531 & 151 & 32273 \\
        player & 85474 & 1254 & 615717 \\
        rabbit & 1558 & 313 & 33961 \\
        stock & 1128 & 143 & 34058 \\
        zebra & 1378 & 99 & 22331 \\
        \bottomrule
    \end{tabular}}
    \label{tab:data_for_each_class}
\end{wraptable}

Our dataset exhibits substantial variability in the number of frames, objects, and boxes across classes, underscoring its diversity as shown in Table \ref{tab:data_for_each_class}. Classes like "person," encompassing "player" and "athlete," are notably prominent with high counts in all three metrics, reflecting their origin from video data of human-centric activities sourced from GMOT-40 \cite{bai2021gmot}, DanceTrack \cite{sun2022dancetrack}, and SportsMOT \cite{cui2023sportsmot}. These activities span a wide array of human motions in various settings. Conversely, "ant" and "bee" classes, falling under "insect," have lower metrics, indicating less frequency or shorter sequence presence. Furthermore, our dataset emphasizes benchmarking across both broader and more specific class subsets, involving 244 "superset" and 286 "subset" queries to refine model accuracy and mitigate category imbalance.

G$^2$MOT integrates GMOT-40, AnimalTrack, DanceTrack, and SportMOT datasets, presenting unique GMOT challenges, as shown in Figure \ref{fig:all_infos}. Specifically, SportMOT focuses on tracking across long gaps and differentiating similar appearances, a task complicated by uniform attire and small, distant objects. It notably features the highest subset-to-superset ratio, challenging object localization based on minor visual differences, as evidenced by the performance impact on re-identification methods detailed in Table \ref{tb:detection_phase}. While SportMOT and GMOT-40 highlight significant movement, DanceTrack is marked by increased occlusion, and both GMOT-40 and AnimalTrack offer a variety of small, similarly appearing objects with a high average object count per frame.

\begin{figure*}
    \centering
    \vspace{-10}
    \includegraphics[width=\textwidth]{figures/supp/[sup]dataset_overview.pdf}
    \caption{All information from each sub-dataset (GMOT-40, AnimalTrack, DanceTrack, SportMOT) for the construction of our G$^2$MOT dataset.}
    \label{fig:all_infos}
\end{figure*}

\hl{We also provide metrics for evaluating our dataset that highlight our contribution, as shown in Table 1,2 in the main paper. To calculate metrics Obj., App., Den., Occ., Mot, for simplicity, let's consider it over one video, where N is the number of frames in the video, the results are mean and std of the following sets:}

    Obj = $\{M^t | \text{ } \forall t, 1 \leq t \leq N\}$, where $M^t$ is the number of objects of frame $t$.

    App = $\{cos<F(O_i^t), F(O_j^t)> |  \text{ } \forall t, 1 \leq t \leq N;  \forall (i,j), i < j < M^t \}$, where $F(.)$ is a pre-trained re-ID model \cite{sun2022dancetrack} to extract appearance embeddings, $O_i^t$ is a object $O_i$ on a frame $t$.

    Occ = $\{IoU(O_i^t, O_j^t) | \text{ } \forall t, 1 \leq t \leq N;  \forall (i,j), i < j < M^t\}$

    Mot = $\{IoU(Track_i^t, Track_i^{t+1}) | \text{ } \forall i, 1 \leq i \leq K ; \forall t, 1 \leq t \leq length(Track_i) - 1 \leq N - 1  \}$. K is the number of tracks in the video, and $Track_i$ is a track corresponding to a track ID throughout the video.

    Den = $\{ Max(H^t) | \text{ } \forall t, 1 \leq t \leq N \}$. $H^t$ is a density heatmap, with each element $H^t[i,j]$ represents the number of objects belonging to pixel $[i,j]$

\section{Kalman+}
\label{sec:kalman}
\subsection{Insight Analysis}
Object Tracking involves the use of videos to track tasks under various conditions such as low frame rates, significant camera movement, and large object deformation. These conditions can introduce noise to the estimators and particularly impact linear estimators such as the Kalman Filter. While the Kalman Filter estimator assesses the state uncertainty covariance, many Kalman Filter-based trackers primarily rely on their own predictions of the next state in the future frame during the object association phase. In this process, the uncertainty covariance is overlooked and typically only involved in calculating the Kalman Gain. To simplify the use of uncertainty covariance, we leverage it to enhance the second-phase matching of KAMSORT, which initially relies solely on the IoU score and observing the effectiveness shown in Table \ref{tab:ablation} and Figures \ref{fig:fig_trackers_compare}, \ref{fig:fig_trackers_compare_2}

\section{Additional Qualitative Comparison}
\label{sec:quali}

\begin{figure*}[h]
    \centering
    \includegraphics[width=\linewidth]{figures/supp/[supp]trackers_compare2.pdf}
    \caption{Comparison of our tracker KAMSORT  with OC-SORT and DeepOCSORT on video insect-3}
    \label{fig:fig_trackers_compare_2}
\end{figure*}

To demonstrate our trackers' effectiveness, we highlight two scenarios: 1) re-associating similar visual cues after a gap, and 2) tracking fast-moving objects for efficiency in both association phases. In Figure \ref{fig:fig_trackers_compare}, DeepOCSORT faces confusion between objects with IDs 1 and 6 due to high occlusion, leading to shared features. Relying solely on appearance similarity scores can introduce errors, especially with unreliable appearance cues, influenced by ReID model robustness. Unreliable appearance cues may impact results, overshadowing IoU (motion cues) contribution.

To improve the flexibility of information processing within the tracker, we have developed a balancing algorithm. This algorithm prioritizes motion over appearance when the visual appearances of all detections are very similar, as described in detail in Section 4 (main paper). As a result, in scenarios like the one shown in Figure \ref{fig:fig_trackers_compare}, where most people wear identical uniforms and objects are difficult to distinguish, we rely heavily on motion cues to track objects, which ensures consistency of object ID, unlike Deep-OCSORT.

Additionally, as illustrated in Figure \ref{fig:fig_trackers_compare_2}, our tracker excels in maintaining ID consistency. Notably, ID 7 consistently remains on the leftmost, and ID 6 consistently remains in the rightmost position from the initial frame. This impressive feat is accomplished through the incorporation of uncertainty revised in the second-phase matching, ensuring the reliable tracking of fast-moving objects or objects in low fps scenarios. It's worth highlighting that, in contrast to the challenges faced by OC-SORT and Deep-OCSORT in linking detections to tracklets, our tracker stands out by avoiding the generation of new identities for objects or discarding them as unstable tracklets.

\section{Discussion on Grounded GMOT}
